# Supplementary material for: DeCoTR: Enhancing Depth Completion with 2D and 3D Attentions
Source: arXiv:2403.12202 source file (2024-03-18)
Supplement: Supplementary file 1 [file 7_suppl.tex]

\clearpage
\setcounter{page}{1}
\maketitlesupplementary

\section*{Depth Evaluation Metrics}
\label{sec:evaluation}
Here we provide the formal definitions for the depth evaluation metrics mentioned in Section 4.1 in our paper.
\begin{align*}
    \text{Abs Rel: } &\frac{1}{N}\sum_{i=1}^N\frac{|d_i - d_i^{*}|}{d_i^{*}},\\
    \text{MAE: }&\frac{1}{N}\sum_{i=1}^N|d_i - d_i^{*}|,\\
    \text{RMSE: }&\sqrt{\frac{1}{N}\sum_{i=1}^N\big|d_i - d_i^{*}\big|^2},\\
    \text{iMAE: }&\frac{1}{N}\sum_{i=1}^N\Big|\frac{1}{d_i} - \frac{1}{d_i^{*}}\Big|,\\
    \text{iRMSE: }&\sqrt{\frac{1}{N}\sum_{i=1}^N\Big|\frac{1}{d_i} - \frac{1}{d_i^{*}}\Big|^2},\\
    \delta < t\text{: }&\frac{M}{N}, \text{ }M=\sum_{i=1}^N\textbf{1}_{\{\delta_i < t\}},\text{ } \delta_i = \max\bigg(\frac{d_i}{d_i^*}, \frac{d_i^*}{d_i}\bigg),
\end{align*}
where $d_i$ is per-pixel predicted depth and $d_i^{*}$ is the ground truth. $N$ is the total number of pixels per each depth map $D=\{d_i\}_{i=1}^N$.  \textbf{1}$_{\{\cdot\}}$ is the indicator function. $t$ is the threshold which takes three values of $1.25$, $1.25^2$ and $1.25^3$. 

\begin{comment}
\section{Rationale}
\label{sec:rationale}
% 
Having the supplementary compiled together with the main paper means that:
% 
\begin{itemize}
\item The supplementary can back-reference sections of the main paper, for example, we can refer to \cref{sec:intro};
\item The main paper can forward reference sub-sections within the supplementary explicitly (e.g. referring to a particular experiment); 
\item When submitted to arXiv, the supplementary will already included at the end of the paper.
\end{itemize}
% 
To split the supplementary pages from the main paper, you can use \href{https://support.apple.com/en-ca/guide/preview/prvw11793/mac#:~:text=Delete%20a%20page%20from%20a,or%20choose%20Edit%20%3E%20Delete).}{Preview (on macOS)}, \href{https://www.adobe.com/acrobat/how-to/delete-pages-from-pdf.html#:~:text=Choose%20%E2%80%9CTools%E2%80%9D%20%3E%20%E2%80%9COrganize,or%20pages%20from%20the%20file.}{Adobe Acrobat} (on all OSs), as well as \href{https://superuser.com/questions/517986/is-it-possible-to-delete-some-pages-of-a-pdf-document}{command line tools}.
\end{comment}
